# Supplementary material for: AI-Enabled Conversational Journaling for Advancing Parkinson's Disease Symptom Tracking
Source: arXiv:2503.03532 source file (2025-03-05)
Supplement: Supplementary file 1 [file 10-appendix.tex]

\section{Gricean Maxims of Cooperative Conversation}
\label{app:grice}
Gricean Maxims are foundational principles that guide cooperative and effective communication in conversational exchanges~\cite{grice1975}. These maxims--Quantity, Quality, Relation, and Manner outline the expectations for how participants should contribute information in a way that fosters clarity, relevance, and truthfulness in dialogue.

\pheading{Maxim of Quantity: The Principle of Optimal Information Disclosure.} Conversation should strive for optimal informativeness in a communicative exchange. This involves delivering a degree of information that is neither excessively detailed nor insufficient but rather commensurate with the requirements of the ongoing discourse. 

\pheading{Maxim of Quality: The Imperative for Veracity and Evidential Support.} This maxim underscores the ethical obligation for speakers to uphold truthfulness throughout the conversational exchange. Participants should refrain from disseminating misinformation or statements believed to be false unless there exists a compelling rationale for such dissemination. If such information must be included, a disclaimer surrounding said information should accompany its presentation.

\pheading{Maxim of Relation: Navigating Relevance in Conversational Context.} Also referred to as the \textit{Maxim of Relevance}, this maxim advises the participants in a conversation to contribute statements that are germane to the ongoing conversational topic~\cite{sperber1986relevance}. Extraneous details should be omitted to maintain focus and coherence. Redirecting conversational drift through follow-up inquiries can serve as an effective mechanism to steer the discussion back to the current topic of discussion.

\pheading{Maxims of Manner: Clarity and Conciseness in Discourse.} 
This maxim emphasizes not merely the content of the communication but also its form. The maxim advocates for clarity and conciseness in language use, cautioning against ambiguous language that could obfuscate meaning. While the preceding maxims largely address the \textit{what} of conversational interaction, the Maxim of Manner focuses on the \textit{how}, endorsing explicit requests for clarification or additional context to support smooth and effective dialogue turns.

\section{Core Design Considerations and Criteria}
\label{app:design_considerations}
Drawing on prior research~\cite{setlur2022you, jovanovic2020chatbots} on conversational agents, as well as extensive discussions with our team, we identified three core considerations that guided our design of \toolname{}: 1) adherence to tenets of cooperative conversation between AI agents and people, 2) the ability to simulate the clinical interview process by generating timely, relevant, and personalized follow-up questions, and 3) enhanced accessibility and ease of use. In the following sections, we detail how these principles were transformed into practical and actionable design considerations.

\subsection{Adherence to tenets of cooperative conversation between AI agents and people}
Drawing from prior work in this area~\cite{setlur2022you}, we devised design criteria (DC) 1 to 4 that govern the journaling agent's conversational behavior in relation to the four maxims.

\begin{tight_itemize}
    \item \noindent\textbf{DC-1: Provide clear conversation initiation \& termination.} 
   The greeting from the conversational agent should be clear, serving as an explicit signal to commence the conversation and guiding the user in knowing when to begin recording their symptoms.

   \hspace{\parindent} \scstart{agent} \textit{``Hi, [name]! Your journal is ready. What would you like to record?''}
    
    \hspace{\parindent} \scstart{human} \textit{``My tremors.''}

    Before terminating the conversation, the conversational agent should ask for confirmation from the user (Maxim of Manner).
    
   \hspace{\parindent} \scstart{agent} \textit{``Is there anything else you'd like to record?''}
    
    \hspace{\parindent} \scstart{human} \textit{``No''}
    
    \hspace{\parindent} \scstart{agent} \textit{``If you need to chat in the future, say ``Alexa, open my Parkinson's journal," and I will assist you in your journaling. Bye!''}

    \item \noindent\textbf{DC-2: Offer relevant acknowledgements.} 
    The conversational agent should provide appropriate and relevant acknowledgments to the user input (Maxims of Quality, Relevance, and Manner).

   \hspace{\parindent} \scstart{human} \textit{``I've been experiencing tremors on and off for a while''}
    
    \hspace{\parindent} \scstart{agent} \textit{``Noted. Can I ask you a few questions about your tremors?''}

    \item \noindent\textbf{DC-3: Support effective transitions between topics.}
The conversational agent should ensure proper topic-switching between the topics and the sub-topics (Maxims of Relevance and Manner).
If the user desires to switch topics or continue the conversation on a new sub-topic, the conversational agent should first ask for the user's acknowledgment and confirm the switch. If the previous topic has an unresolved question, the agent should clarify if the user wants to resolve the question before moving to another topic. This ensures a smooth transition of topics and sub-topics by requesting user acknowledgment and clarification when switching~\cite{skantze2021turn, jiang2023communitybots}.

   \hspace{\parindent} \scstart{agent} \textit{``When did you take your Parkinson's medication?''}
   
    \hspace{\parindent} \scstart{human} \textit{``I don't want to talk about my medication. I didn't get complete sleep last night.''} 
    
    \hspace{\parindent} \scstart{agent} \textit{``I am sorry to hear that. Can I ask you a few questions about your lack of sleep?''} 
    
    \hspace{\parindent} \scstart{human} \textit{``Yes!''} 
    
    \hspace{\parindent} \scstart{agent} \textit{``How long could you sleep last night?''}

     \item \noindent\textbf{DC-4: Provide conversation repair \& refinement.}The system should provide timely repair and refinement related to issues such as breakdowns in the flow of conversation due to misunderstandings, misinterpretations, technical glitches, or user dissatisfaction (Maxims of Relevance and Quality). Conversation repair involves identifying and resolving these issues to ensure the conversation continues smoothly and effectively \cite{ashktorab2019resilient, setlur2022you}. The system should also provide refinement by improving or enhancing the quality of the interaction. For instance, clarifying ambiguous statements, providing additional information, or making the conversation more engaging and user-friendly \cite{setlur2022you, chan2022challenges}.

   \hspace{\parindent} \scstart{agent} \textit{``Did you take your prescribed medication?''}
    
    \hspace{\parindent} \scstart{human} \textit{``What medication?''} 
    
    \hspace{\parindent} \scstart{agent} \textit{``Your prescribed levodopa medication.''}
    
\end{tight_itemize}

Design criteria $DC1-4$ are domain and activity-agnostic, applicable to most conversational agents. However, conversing with people about their health is an intimate and sensitive activity that requires additional careful considerations. In this work, we particularly considered four factors: security, empathy, understanding of Parkinson's-related medical terminology, and avoiding giving medical advice. Ensuring security is crucial to protect sensitive patient information from unauthorized access and breaches. Avoiding unsolicited medical advice is essential to prevent misguiding patients and ensure they receive accurate information from qualified healthcare providers. Incorporating empathy in healthcare conversational agents has been associated with positive outcomes such as building trust, increasing patient engagement, and providing psychological support~\cite{adikari2022empathic,daher2020empathic,devaram2020empathic}. Understanding medical terminology is critical for accurate intent identification and the generation of follow-up questions.

\begin{tight_itemize}
    \item \noindent\textbf{DC-5: Implement security measures.} 
    The conversational agent should implement strong privacy and security measures to protect the users' entries and support end-to-end encryption, especially if sensitive information is involved. This design consideration should be supported as part of the conversational agent's backend implementation.

    \item \noindent\textbf{DC-6: Integrate empathy in the agent responses.} 
    The conversational agent should incorporate empathy in their responses (Maxim of Manner). 
    
    \hspace{\parindent} \scstart{human} \textit{``My tremors are worse today''} 
    
    \hspace{\parindent} \scstart{agent} \textit{``I am sorry to hear that! Can I ask you a few questions about your tremors?''}
    
    \item \noindent\textbf{DC-7: Understand medical terminology.} 
    The agent should recognize medical terminology and alternative lay-language terms that the user could use. For the scope of our work, this design consideration concerns Parkinson's disease.
    
   \hspace{\parindent} \scstart{human} \textit{``My fingers and hands were very shaky this morning.''}
    
    \hspace{\parindent} \scstart{agent} \textit{``I am sorry to hear that. It seems like you are experiencing tremors. Can I ask you a few follow-up questions?''} 

 \item \noindent\textbf{DC-8: Refrain from providing healthcare advice.} 
    The conversational agent should refrain from providing explicit or implicit clinical or general healthcare advice to the patient.

    \hspace{\parindent} \scstart{human} \textit{``Do you know any homemade remedies for insomnia?''}
    
    \hspace{\parindent} \scstart{agent} \textit{``I'm sorry I can only assist you with journaling. I can not provide any medical insights or advice. Please consult your healthcare provider if you need  help.''} 
    
\end{tight_itemize}

\subsection{Ability to simulate the clinical interview process by generating timely, relevant, and personalized follow-up questions}
A key element of the conversational journaling paradigm is being able to ask timely and relevant follow-up questions. Conversation personalization, such as using the patient's name and referencing their medical history, can enhance the patient experience by building trust and increasing the relevance of the information provided~\cite{liu2022roles, liu2022effects, kocaballi2019personalization}.
 
  \begin{tight_itemize}

         \item \noindent\textbf{DC-9: Generate relevant and timely follow-up questions.} 
             The follow-up questions should be contextually relevant and timely, aiming to elicit additional information from the user's input.

             \hspace{\parindent} \scstart{human} \textit{``My joints pain was worse this afternoon.''}
   
            \hspace{\parindent} \scstart{agent} \textit{``When did you last take your pain medication?''}

         \item \noindent\textbf{DC-10: Support personalization.} 
              The conversational agent should use conversation history to personalize the content and the delivery of the conversation as much as possible.
    
            \hspace{\parindent} \scstart{agent} \textit{``[name], How your tremors compare to those you mentioned last week?''}
   
            \hspace{\parindent} \scstart{human} \textit{``They are about the same.''} 

    \end{tight_itemize}

$DC-9$ led us to ask two critical questions: (1) What expressions in PwPD utterances should trigger follow-up questions? and (2) What additional information would be valuable to collect? To address these questions, we collaborated closely with our team's neurologist. Based on their recommendations, we selected six prevalent Parkinson's symptoms—\textit{tremors}, \textit{bradykinesia}, \textit{loss of balance/dizziness}, \textit{falls}, \textit{mood/emotion}, and \textit{sleeplessness}—as triggers for follow-up questions. Focusing on these prevalent symptoms ensured the system's relevance to a broad range of PwPD. Additionally, the neurologist recommended $10$ ``probing topics''  for which collecting additional information could increase the clinical value of journaling. The probing topics include \textit{medication}, \textit{daily activity}, \textit{severity}, \textit{cooccurence}, \textit{duration}, \textit{time of day}, \textit{location}, \textit{activity at the time}.
\textit{trigger factors}, and \textit{history}. For Parkinson's symptoms outside our pre-selected set (e.g., speech problems) or other issues expressed by the patient (e.g., missing workout), \toolname{} records and acknowledges the symptom or issue but does not issue any follow-up questions. Table~\ref{tab:sympthoms_and_topics} presents the selected symptoms, probing topics, example follow-up questions, and their interrelationships.

Identification of one of the six symptoms (e.g., tremor) by \toolname{} would initiate the process of generating and asking a relevant follow-up question. It is important to note that the mapping between probing topics and symptoms is not one-to-one. The set of follow-up questions generated depends on the detected symptom. For instance, the system will not follow up with a question about ``duration'' if the detected symptom is ``falling''. Conversely, the question about the ``duration'' will be asked upon detection of ``tremor'' or ``dizziness'' in the patient's utterance.

\subsection{Enhanced accessibility and ease of use}
The final design criteria emphasize employing mechanisms that make access and use of \toolname{} easier, particularly for PwPD who may experience motor function issues. This focus aimed to accommodate those who might struggle with GUI-based or physical data entry methods, ensuring that \toolname{} remains accessible and user-friendly for all users. 

\begin{itemize}
 \item \noindent\textbf{DC-11: Enable low-barrier and accessible journaling support.} 
            The journaling should be made accessible and delivered in a way that requires minimal physical and cognitive demand.
            For instance, the conversational agent should be accessible on low-barrier smart devices such as smart speakers via voice. 
\end{itemize}

\section{Participants}
\label{app:pre_study_questions}
The demographic information about the participants from Study I and II collected using the pre-study questionnaire are shown in Tables~\ref{tab:participants_1} and \ref{tab:participants_2} respectively.

\begin{table*}[!ht]
  \centering
  \caption{Study I participants.}
  \label{tab:participants_1}
  
    \includegraphics[width=\linewidth]{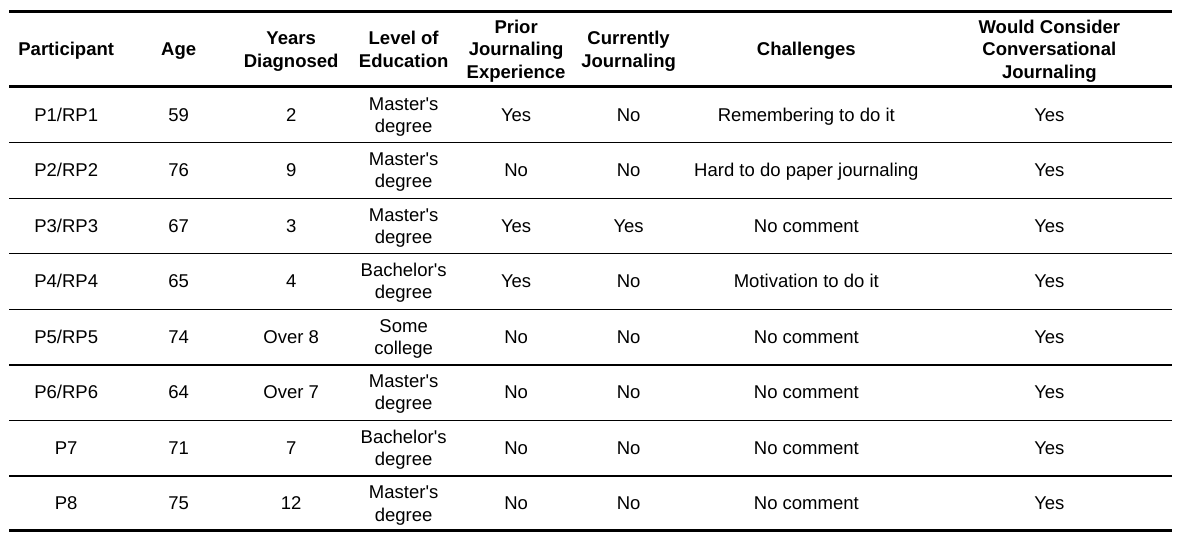} 
    
\end{table*}

\begin{table*}[!ht]
  \centering
  \caption{Newly recruited participants for Study II.}
  \label{tab:participants_2}
  
    \includegraphics[width=\linewidth]{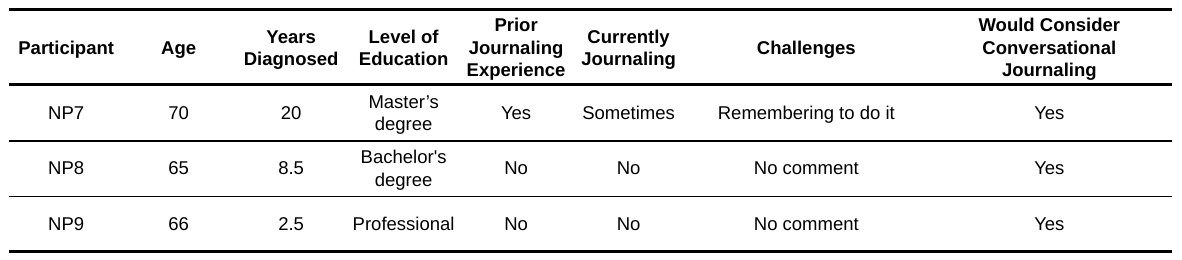} 
    
\end{table*}

\section{Post-study Questionnaire}
\label{app:post_study_questions}
The list of post-study questions asked to the participants are shown in Table~\ref{tab:post_study}.

\begin{table*}[t]
  \centering
  \caption{This table shows the list of post-study questions.}
  \label{tab:post_study}
  
    \includegraphics[width=\linewidth]{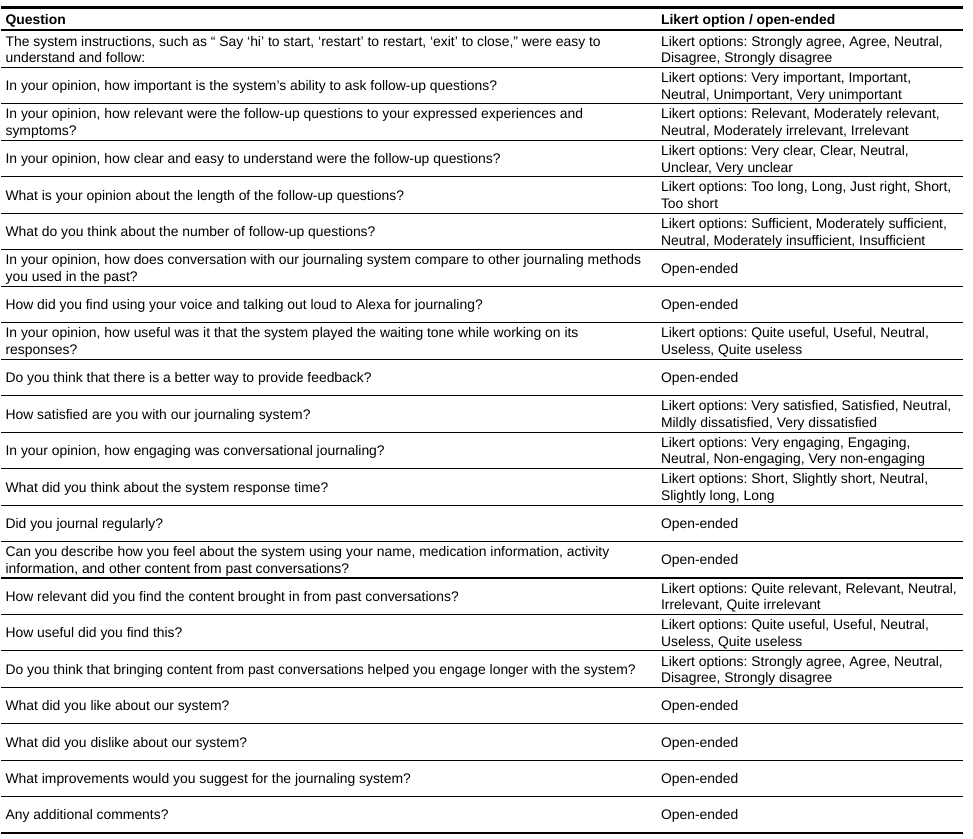} 
    
\end{table*}

\section{LLM Prompt for Personalization}
\label{app:llm_personalization}

To prompt the LLM for personalization, we segmented the user's conversation log into three components: ``conversation context,'' ``profile,'' and ``conversation history.'' 
The conversation context includes the exchanges between the user and \toolname{} in the current session, which we define as a single continuous interaction from start to finish. 
The profile contains the user's name, medication details, daily activities, and challenges with Parkinson's.
The profile information is recorded only once during the initial session with \toolname{}. 
The conversation history contains all past exchanges between the user and \toolname{}, excluding the profile and current conversation context. Given the conversation context, profile, history, and the latest message between a user and \toolname{}, we used the following prompt for personalization:\\

\begin{mdframed}
\highlight{\textbf{Prompt:}} \textit{``Imagine you are a chatbot, and the following is the conversation between you and a user: + [conversation context] + Also, you are given the following profile of the user who is a Parkinson's patient: + [profile] + And the following conversation history between you and the user: + [conversation history] + Your latest utterance is: [latest user message] + Now use relevant and appropriate content from the conversation, history, and the profile of the user, including their medication intake and time, daily activities, prior reported symptoms, and so on, to paraphrase and personalize the latest message. Make the personalized utterance sound natural and coherent to the conversation. Don't say anything else.''}
\end{mdframed}

\section{Analysis for System Improvement}

\subsection{Evaluating LLMs for Intent Identification}
\label{app:expt1_intent}

\begin{table}[!ht]
    \centering
    \caption{The table shows the results of our experiments evaluating the performance of GPT-4, FlanT5-XXL, and Meditron-7B in intent prediction using data from Experiment I. We show the performance of these models across the eight participants of Experiment I.}
    \includegraphics[width=\textwidth]{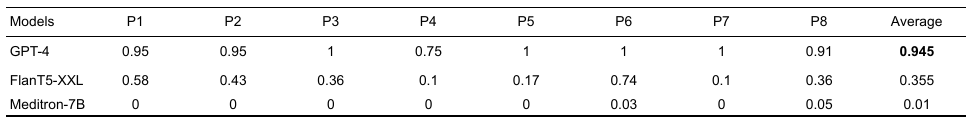}
    \label{tab:llm_intent_expt1}
\end{table}

Table~\ref{tab:llm_intent_expt1} presents the results of our experiments on intent prediction using LLMs. We utilized data from Experiment I and tested three LLMs: GPT-4, FlanT5-XXL, and Meditron-7B. The results from our experiment showed that GPT-4 achieved higher performance with an accuracy of 95\%. 
In contrast, FlanT5-XXL and Meditron-7B demonstrated significantly lower accuracies of 36\% and 1\%, respectively.
We used the following prompt for all three models:\\

\begin{mdframed}
\highlight{\textbf{Prompt:}} \textit{``Imagine you are a journaling chatbot who is talking to a Parkinson's patient. The user responded with + [latest user message] + when asked, `What do you want to record?' by the chatbot. Based on the above information, predict the Parkinson's symptoms that the user is experiencing. Answer with the following symptoms: `tremor,' `bradykinesia,' \ldots, `insomnia.' Here are a few examples for each of the symptoms, use them as reference -- `tremor': `my hands have been shaking uncontrollably; my tremors,' `bradykinesia': `I'm moving much slower than usual; slowness in movement,' \ldots, `insomnia': `trouble sleeping at night; can't sleep despite being tired.' If the user reports more than one symptom, say \'multiple\.' If the user message contains an audio speech recognition error, for instance, incomplete sentences and ambiguous words, say, `asr'. If the user did not mention any symptom or their response says they are not experiencing anything, say `none'. Don't use quotes. Don't say anything else.''}
\end{mdframed}
